# Supplementary material for: A Geometric Perspective towards Neural Calibration via Sensitivity Decomposition
Source: arXiv:2110.14577 source file (2021-11-21)
Supplement: Supplementary file 1 [file cifar100_noise_appendix.tex]

\begin{table*}
\centering
\resizebox{1.0\linewidth}{!}{%
\begin{tabular}{c|ccccc|ccccc|ccccc}  
\toprule
& \multicolumn{5}{c}{ECE$\downarrow$} & \multicolumn{5}{c}{NLL$\downarrow$}&  \multicolumn{5}{c}{Brier$\downarrow$}\\
\midrule
Noise-level& 1&2&3&4&5 & 1&2&3&4&5& 1&2&3&4&5 \\
\midrule
Ensemble &\textbf{0.059} &\textbf{0.076} &\textbf{0.078} &\textbf{0.107} &\underline{0.149} 
         &\textbf{1.499} &\textbf{1.927} &\textbf{1.969} &\textbf{2.379} &\textbf{2.99} 
         &0.005 &0.006 &0.006 &0.007 &0.008 
         
\\
MCDO &0.114$\pm$0.002 &0.147$\pm$0.002 &0.14$\pm$0.006 &0.192$\pm$0.009 &0.255$\pm$0.014 
     &1.789$\pm$0.011 &2.225$\pm$0.012 &\underline{2.236$\pm$0.043} &2.788$\pm$0.072 &3.585$\pm$0.119 
     &0.005$\pm$0.0 &0.006$\pm$0.0 &0.006$\pm$0.0 &0.007$\pm$0.0 &0.009$\pm$0.0 
     \\
\midrule
ResNet &0.113$\pm$0.004 &0.149$\pm$0.005 &0.152$\pm$0.004 &0.185$\pm$0.005 &0.237$\pm$0.01 
       &\underline{1.782$\pm$0.018} &2.269$\pm$0.023 &2.326 $\pm$ 0.029 &2.773$\pm$0.027 &3.434$\pm$0.032 
       &0.005$\pm$0.0 &0.006$\pm$0.0 &0.007$\pm$0.0 &0.007$\pm$0.0 &0.009$\pm$0.0 
       \\

\midrule
Ours &\underline{0.067$\pm$0.002} &\underline{0.083$\pm$0.002} &\underline{0.089$\pm$0.004} &\underline{0.116$\pm$0.007} &\textbf{0.145$\pm$0.013}
     &1.786$\pm$0.013 &\underline{2.208$\pm$0.013} &2.300$\pm$0.014 &\underline{2.676$\pm$0.015} &\underline{3.215$\pm$0.028}
     &\textbf{0.003$\pm$0.0} &\textbf{0.005$\pm$0.0} &\textbf{0.006$\pm$0.0} &\textbf{0.007$\pm$0.0} &\textbf{0.008$\pm$0.000}
     \\
     
\bottomrule
\end{tabular}}
\caption{\textbf{ResNet18 on CIFAR100 Noise}, averaged over 5 seeds}
\label{tab:cifar100_noise_appendix}
\vspace{-5mm}
\end{table*}
