# Supplementary material for: A Geometric Perspective towards Neural Calibration via Sensitivity Decomposition
Source: arXiv:2110.14577 source file (2021-11-21)
Supplement: Supplementary file 2 [file cifar10_noise_appendix.tex]

\begin{table*}
\centering
\resizebox{1.0\linewidth}{!}{%
\begin{tabular}{c|ccccc|ccccc|ccccc}  
\toprule
& \multicolumn{5}{c}{ECE$\downarrow$} & \multicolumn{5}{c}{NLL$\downarrow$}&  \multicolumn{5}{c}{Brier$\downarrow$}\\
\midrule
Noise-level& 1&2&3&4&5 & 1&2&3&4&5& 1&2&3&4&5\\
\midrule
Ensemble &\underline{0.051} & \underline{0.075} & \underline{0.076} & \underline{0.118} & \underline{0.184} 
         &\underline{0.544} & \underline{0.737} &\textbf{0.753} &\underline{1.055} &\underline{1.551} 
         &\textbf{0.021} &\textbf{0.028} &\textbf{0.03} &\textbf{0.041} &\underline{0.057} 
        
\\
MCDO     &0.076$\pm$0.003 &0.098$\pm$0.004 &0.102$\pm$0.002 &0.164$\pm$0.005 &0.251$\pm$0.008 
         &0.667$\pm$0.02 &0.845$\pm$0.029 &0.831$\pm$0.013 &1.262$\pm$0.033 &1.947$\pm$0.054 
         &0.024$\pm$0.0 &0.03$\pm$0.001 &0.032$\pm$0.0 &0.046$\pm$0.001 &0.065$\pm$0.001 
         \\
\midrule
ResNet &0.102$\pm$0.001 &0.141$\pm$0.003 &0.153$\pm$0.007 &0.209$\pm$0.011 &0.293$\pm$0.016 
       &0.718$\pm$0.01 &0.979$\pm$0.019 &1.043$\pm$0.046 &1.436$\pm$0.081 &2.052$\pm$0.133 
       &0.025$\pm$0.0 &0.034$\pm$0.0 &0.038$\pm$0.001 &0.05$\pm$0.002 &0.068$\pm$0.002 \\

\midrule
Ours &\textbf{0.040$\pm$0.002} &\textbf{0.055$\pm$0.003} &\textbf{0.060$\pm$0.005} &\textbf{0.080$\pm$0.01} &\textbf{0.106$\pm$0.012}
     &\textbf{0.531$\pm$0.006} &\textbf{0.716$\pm$0.012} &\underline{0.785$\pm$0.013} &\textbf{1.007$\pm$0.018} &\textbf{1.346$\pm$0.02}
     &\underline{0.022$\pm$0.0} &\underline{0.03$\pm$0.0} &\underline{0.034$\pm$0.0} &\underline{0.043$\pm$0.001} &\textbf{0.056$\pm$0.001}
    \\
\bottomrule
\end{tabular}}
\caption{\textbf{ResNet18 on CIFAR10 Noise}, averaged over 5 seeds}
\label{tab:cifar10_noise_appendix}
\vspace{-5mm}
\end{table*}
